# Supplementary material for: Thermodynamic Limits of Photon-Multiplier Luminescent Solar Concentrators
Source: arXiv:2203.06736 source file (2022-03-13)
Supplement: Supplementary file 1 [file SI.pdf]

# Supplemental Material
# for Thermodynamic Limits of Photon-Multiplier Luminescent Solar Concentrators

Tomi K. Baikie, Arjun Ashoka, Akshay Rao, and Neil C. Greenham*
*Cavendish Laboratory, University of Cambridge, Cambridge, CB3 0HE, UK*

## SUPPLEMENTAL MATERIAL

### A. Terrestrial Conditions

For a traditional LSC, the concentration limit is given by Equation 10. To determine the concentration limit under terrestrial conditions, one may integrate over the solar spectrum and over the luminescence spectrum as a function of frequency to determine the ratio of $B_1$ and $B_2$. In the case of the PM-LSC (Equation 12 in the main text), the concentration limit remains brightness dependent. It is of general interest to relate this expression to a terrestrial environment.

SI Figure 1 plots the spectral irradiance given by the ASTM G-173-03 standard [1]. The integrated power density is 1000.38 Watts per unit area. Assuming the bandgap of silicon is 1.12 eV (dashed line), the lowest energy photon the PM material could absorb is 2.24 eV, corresponding to a photon wavelength of 553 nm (dash-dot line). The shaded area indicates the absorbed photons. The integrated absorbed power density is 268 Watts per unit area. This corresponds to a photon flux of $6 \times 10^{20}$ photons per second per unit area.

For Figure 2 we assume that all photons arrive at frequency $\nu_1$ at a fixed brightness matching that of the absorbed solar flux that is in equilibrium with the chromophore. Notably, depending over the bandwidth range that $\nu_1$ is absorbed over, the brightness we approximate may change by several orders of magnitude. In reality, each frequency slice of the incoming solar irradiation should have a corresponding brightness. However, to highlight the effect of the free energy change on the concentration limit by exciting beyond the band edge, we assume some fixed and narrow finite bandwidth. A finite amount of radiation contains always a finite, although possibly very narrow, range of the spectrum. This range will determine the brightness of the beam.

The relevant frequency bandwidth to use is not obvious to us, and may be somewhat arbitrary when compressing solar radiation to some fixed bandwidth in any case. If the spectrum were remains unmodified, and over the entire absorption range, this would result in a bandwidth of $1 \times 10^{15}$ Hz and thus a brightness of $1 \times 10^{6}$ photons per second per unit bandwidth per unit area per $4\pi$ solid angle. If the solar energy absorbed is quickly thermalised and then distributed by ambient thermal energy on the order of $(k_B T) \sim 0.026$ eV, this would result in a bandwidth of $1 \times 10^{12}$ Hz and a brightness on the order of $1 \times 10^{9}$ photons per second per unit bandwidth per unit area per $4\pi$ solid angle.

In the PM-LSC case, as the brightness decreases, the maximum concentration factor increases. Here, based on the ambient thermal energy argument, we assume a brightness on the order of $1 \times 10^{9}$ photons per second per unit bandwidth per unit area per $4\pi$ solid angle, which we treat as a reasonable lower bound.

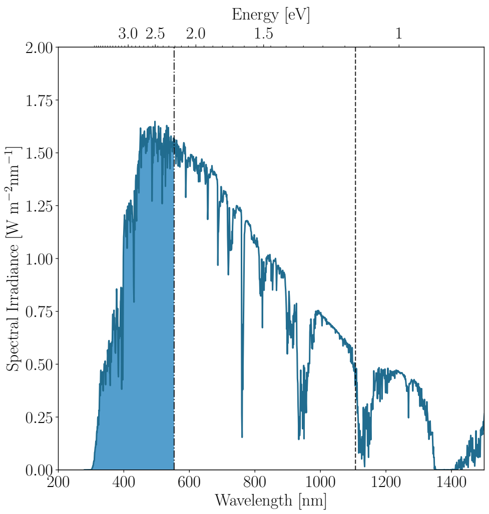


SI Fig. 1. **Terrestrial spectral irradiance**. The dashed black line at 1107 nm corresponds to the the bandgap of a silicon solar cell. The dash-dot line at 553 nm corresponds to the lowest energy photon a silicon solar cell optimised photon multiplier may absorb. The integral of the blue region returns an integrated absorbed power density of 268 Watts per unit area.

### B. Entropy Approximation

SI Figure 2 plots the entropy per photon as a function of brightness for photons of wavelength $\lambda = 500$ nm. Entropy per photon is divided by $k_B$. The red line is our approximation, where entropy per photon is given as

$$s = \ln\left(\frac{8\pi n\nu^2}{c^2 B}\right), \tag{SI 1}$$

and the blue line is the full form,

* ncg11@cam.ac.uk

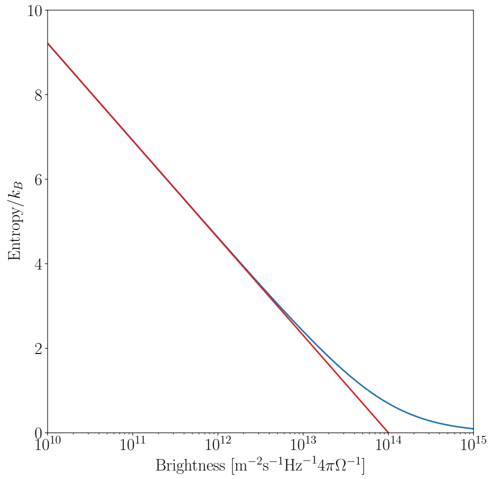


SI Fig. 2. **Entropy per photon divided by $k_B$ as a function of brightness**. The red line is our approximation (Equation SI 1) and the blue line is the full form (Equation SI 2).

$$s = \ln\left(1 + \frac{8\pi n\nu^2}{c^2 B}\right). \quad \text{(SI 2)}$$

The assumption diverges from around brightness $10^{13}$ photons per unit area per unit bandwidth per second per $4\pi$ solid angle.

### C. Efficiency Dependent Expression

The concentration ratio can be written as a function of PM efficiency, $\gamma$, where $1 \leq \gamma \leq 2$,

$$C(\gamma) = \left(\left(\frac{8\pi n^2}{c^2}\right)^{(\gamma-1)} \frac{1}{B_1^{\gamma-1}} \frac{\nu_2^{2\gamma}}{\nu_1^2} e^{\frac{h(\nu_1-\gamma\nu_2)}{k_B T}}\right)^{\frac{1}{\gamma}} \quad \text{(SI 3)}$$

which reduces to the traditional LSC concentration ratio for $\gamma = 1$ (Equation 10 in the main text), as it should.


[1] NREL, Reference Air Mass 1.5 Spectra.
